# Supplementary material for: Physics-Inspired Generative Models in Medical Imaging: A Review
Source: arXiv:2407.10856 source file (2024-08-23)
Supplement: Supplementary file 1 [file PFGMpp.tex]

\section*{APPENDIX B}
This appendix contains informal mathematical derivations related to PFGM++\cite{xu2023} aimed to enhance the intuition of the interested reader. As stated above, by setting  $p_r(\bm{x}|\bm{y}) \propto 1/(|| \bm{x}-\bm{y}||_2^2+r^2)^{\frac{N+D}{2}}$ we can ensure that the minimizer of Eq. \eqref{pfgmpp_obj_final} is $f^*_\theta(\bm{\tilde{x}}) = \sqrt{D} \bm{E} (\bm{\tilde{x}})_{\bm{x}} \cdot E(\bm{\tilde{x}})_r^{-1}.$ Similar to the proof of Proposition 3.2. \cite{xu2023}, this follows since the minimizer of Eq. \eqref{pfgmpp_obj_final} is 
\begin{equation}
    f^*_\theta(\bm{\tilde{x}}) = \int p_r(\bm{y}|\bm{x})\frac{\bm{x}-\bm{y}}{r/\sqrt{D}} d\bm{y} = \sqrt{D} \frac{\int p_r(\bm{x}|\bm{y})(\bm{x}-\bm{y}) p(\bm{y})d\bm{y}}{rp_r(\bm{x})}.   
    \label{pfgmpp_fstar_step1}
\end{equation}
Now, since $p_r(\bm{x}|\bm{y}) \propto 1/(|| \bm{x}-\bm{y}||_2^2+r^2)^{\frac{N+D}{2}}$ and $p_r(\bm{x})=\int p_r(\bm{x}|\bm{y})p(\bm{y})d\bm{y}$ we can rewrite the right hand side in Eq. \eqref{pfgmpp_fstar_step1} as
\begin{equation}
    \sqrt{D} \frac{\int p_r(\bm{x}|\bm{y})(\bm{x}-\bm{y}) p(\bm{y})d\bm{y}}{\int rp_r(\bm{x}|\bm{y})p(\bm{y})d\bm{y}}
    \propto \sqrt{D} \frac{\int \frac{\bm{x}-\bm{y}}{||\bm{\tilde{x}}-\bm{\tilde{y}}||^{N+D}}p(\bm{y})d\bm{y}}{\int \frac{r}{||\bm{\tilde{x}}-\bm{\tilde{y}}||^{N+D}}p(\bm{y})d\bm{y}} 
    = \sqrt{D} \bm{E} (\bm{\tilde{x}})_{\bm{x}} \cdot E(\bm{\tilde{x}})_r^{-1}.  
    \label{pfgmpp_fstar_step2}
\end{equation}

Reference \cite{xu2023} shows that both the training and sampling processes of PFGM++ converge to those of score-based diffusion models (EDM \cite{karras2022}) in the $D\rightarrow \infty, r=\sigma\sqrt{D}$ limit. To build intuition, we provide sketches of these proofs. In particular, we will start by showing that
\begin{equation}
    \lim_{\substack{D\to \infty \\ r=\sigma \sqrt{D}}} \sqrt{D} \bm{E}(\bm{\tilde{x}})_{\bm{x}} / E(\tilde{\bm{x}})_r \propto \sigma \nabla_{\bm{x}}\log p_\sigma (\bm{x}). 
    \label{pfgmpp_obj_limit}
\end{equation}
For formal statements and proofs please see Theorem 4.1 and Proposition 4.2 in \cite{xu2023}. The limit in Eq. \eqref{pfgmpp_obj_limit} is establish by first showing that $p_r(\bm{x}|\bm{y})$ converges to $p_\sigma(\bm{x}|\bm{y})$ in the same limit. Recall that $p_r(\bm{x}|\bm{y})$ is chosen such that $p_r(\bm{x}|\bm{y}) \propto 1/(|| \bm{x}-\bm{y}||_2^2+r^2)^{\frac{N+D}{2}} = (|| \bm{x}-\bm{y}||_2^2+r^2)^{-\frac{N+D}{2}}.$ Taking the limit, we have that
\begin{align}
    \lim_{\substack{D\to \infty \\ r=\sigma \sqrt{D}}} p_r(\bm{x}|\bm{y}) &\propto \lim_{\substack{D\to \infty \\ r=\sigma \sqrt{D}}} (|| \bm{x}-\bm{y}||_2^2+r^2)^{-\frac{N+D}{2}} \propto \lim_{D\to \infty} \exp \left(-\frac{N+D}{2}\log (\frac{|| \bm{x}-\bm{y}||_2^2}{D\sigma^2}+1) \right) \notag \\
    &= \lim_{D\to \infty} \exp \left(-\frac{N+D}{2} \frac{|| \bm{x}-\bm{y}||_2^2}{D\sigma^2}\right) = \exp \left(-\frac{|| \bm{x}-\bm{y}||_2^2}{\sigma^2}\right) \propto p_\sigma (\bm{x}|\bm{y}). 
    \label{perturbation_limit}
\end{align}
Now, using that the right hand side in Eq. \eqref{pfgmpp_fstar_step1} is proportional to Eq. the right hand side in Eq. \eqref{pfgmpp_fstar_step2}, we establish the desired limit as 
\begin{align}
    \lim_{\substack{D\to \infty \\ r=\sigma \sqrt{D}}} \sqrt{D} \bm{E}(\bm{\tilde{x}})_{\bm{x}} / E(\tilde{\bm{x}})_r  &\propto \lim_{\substack{D\to \infty \\ r=\sigma \sqrt{D}}} \sqrt{D} \frac{\int p_r(\bm{x}|\bm{y})(\bm{x}-\bm{y}) p(\bm{y})d\bm{y}}{rp_r(\bm{x})} \notag \\
    &\propto \frac{\int p_\sigma(\bm{x}|\bm{y})\frac{(\bm{x}-\bm{y})}{\sigma} p(\bm{y})d\bm{y}}{p_\sigma(\bm{x})} \propto  \sigma \nabla_{\bm{x}}\log p_\sigma (\bm{x}),
\end{align}
where we used the result from Eq. \eqref{perturbation_limit} Applying a simple change-of-variables via the alignment formula $r=\sigma \sqrt{D}$, using $\sigma:=\sigma(t)=t$, yields the equivalence between $d\bm{x}/dt$ in Eq. \eqref{edm_ode} and $d\bm{x}/dr$ in Eq. \eqref{pfgmpp_ode} Finally, it is possible to show that $\lim_{D \to \infty} p_{r_{\text{max}}=\sigma_{\text{max}}\sqrt{D}} (\bm{x}) = \mathcal{N}(\bm{0},\sigma_{\text{max}}^2\bm{I}).$ Hence, the sampling process of PFGM++ converges to that of diffusion models \cite{karras2022} in the $D \to \infty, r=\sigma\sqrt{D}$ limit. To show the equivalence of the training objectives, we write the weighted denoising score matching objective for the diffusion model as
\begin{equation}
    \mathbb{E}_{\sigma \sim p(\sigma)} \mathbb{E}_{\bm{y}\sim p(\bm{y
    })} \mathbb{E}_{\bm{x}\sim p_{\sigma}(\bm{x}|\bm{y})} \left[\lambda(\sigma)||f_{\theta}(\bm{x},\sigma)-\frac{\bm{x}-\bm{y}}{\sigma}||_2^2\right]. 
    \label{edm_obj_updated}
\end{equation}
The minimizer of this objective is 
\begin{equation}
    f^*_{\theta,\text{DSM}}(\bm{x},\sigma) = \frac{\int p_\sigma(\bm{x}|\bm{y})\frac{(\bm{x}-\bm{y})}{\sigma} p(\bm{y})d\bm{y}}{p_\sigma(\bm{x})} = -\sigma \nabla_{\bm{x}}\log p_\sigma (\bm{x}). 
\end{equation}
Taking the $D \to \infty, r=\sigma \sqrt{D}$ limit
\begin{align}
    \lim_{\substack{D\to \infty \\ r=\sigma \sqrt{D}}} f^*_{\theta,\text{PFGM++}}(\tilde{\bm{x}}) &=  \lim_{\substack{D\to \infty \\ r=\sigma \sqrt{D}}} \sqrt{D} \frac{\int p_r(\bm{x}|\bm{y})(\bm{x}-\bm{y}) p(\bm{y})d\bm{y}}{rp_r(\bm{x})} \\
    &\propto \frac{\int p_\sigma(\bm{x}|\bm{y})\frac{(\bm{x}-\bm{y})}{\sigma} p(\bm{y})d\bm{y}}{p_\sigma(\bm{x})} = f^*_{\theta,\text{DSM}}(\bm{x},\sigma),
\end{align}
where the limit is evaluated using the results from Eq. \eqref{perturbation_limit} In other words, the training objectives of diffusion models \cite{karras2022} and PFGM++ \cite{xu2023}, despite appearing widely different, are in fact equivalent in the $D \to \infty, r=\sigma \sqrt{D}$ limit.
